# Supplementary material for: Beam Asymmetry $\mathbf{\Sigma}$ for the Photoproduction of $\mathbf{\eta}$ and $\mathbf{\eta^{\prime}}$ Mesons at $\mathbf{E_{\gamma}=8.8}$GeV
Source: arXiv:1908.05563 source file (2019-11-24)
Supplement: Supplementary file 1 [file supplemental.pdf]

# BEAM ASYMMETRY Σ FOR THE PHOTOPRODUCTION OF $\eta$ AND $\eta'$ MESONS AT $E_\gamma = 8.8$ GEV: SUPPLEMENTAL MATERIAL

TABLE I. Values and errors for the photon beam asymmetry $\Sigma_\eta$ for the reaction $\gamma p \to \eta p$ with $\eta \to \gamma\gamma$. For the binning in $t$, we report the range of the data, the event-weighted mean of all $t$ values, and the RMS of that distribution. For $\Sigma_\eta$, we report the value, statistical error, and systematic error. The total error is the sum of the previous two in quadrature. Not reported here is the 2.1% relative uncertainty due to the determination of the polarization of the photon beam.

| Binning in $t$ (GeV$^2$) | | | | Uncertainties | | |
|---|---|---|---|---|---|---|
| Range | Mean | RMS | $\Sigma_\eta$ | Statistical | Systematic | Total |
| $0.1 < -t < 0.2$ | 0.153 | 0.028 | 1.039 | 0.037 | 0.035 | 0.052 |
| $0.2 < -t < 0.3$ | 0.248 | 0.029 | 1.009 | 0.036 | 0.025 | 0.045 |
| $0.3 < -t < 0.45$ | 0.369 | 0.043 | 1.000 | 0.035 | 0.021 | 0.042 |
| $0.45 < -t < 0.7$ | 0.559 | 0.071 | 0.948 | 0.036 | 0.016 | 0.040 |
| $0.7 < -t < 1.5$ | 0.964 | 0.206 | 0.865 | 0.038 | 0.025 | 0.046 |

TABLE II. Values and errors for the photon beam asymmetry $\Sigma_{\eta'}$ for the reaction $\gamma p \to \eta' p$ with $\eta' \to \eta\pi^+\pi^-$ and the $\eta \to \gamma\gamma$. For the binning in $t$, we report the range of the data, the event-weighted mean of all $t$ values, and the RMS of that distribution. For $\Sigma_{\eta'}$, we report the value, statistical error, and systematic error. The total error is the sum of the previous two in quadrature. Not reported here is the 2.1% relative uncertainty due to the determination of the polarization of the photon beam.

| Binning in $t$ (GeV$^2$) | | | | Uncertainties | | |
|---|---|---|---|---|---|---|
| Range | Mean | RMS | $\Sigma_{\eta'}$ | Statistical | Systematic | Total |
| $0.1 < -t < 0.3$ | 0.206 | 0.061 | 0.858 | 0.064 | 0.033 | 0.072 |
| $0.3 < -t < 0.5$ | 0.392 | 0.056 | 0.902 | 0.075 | 0.033 | 0.082 |
| $0.5 < -t < 0.7$ | 0.589 | 0.056 | 0.888 | 0.096 | 0.067 | 0.117 |
| $0.7 < -t < 1.2$ | 0.883 | 0.136 | 0.916 | 0.094 | 0.034 | 0.100 |

TABLE III. Values and errors for the ratio of photon beam asymmetries $\Sigma_{\eta'}/\Sigma_{\eta}$ for the reported reactions. To form the ratio, the $\eta$ analysis is done with the same binning in $t$ as the $\eta'$ analysis, and for each bin we report the range of the data, the event-weighted mean of all $t$ values, and the RMS of that distribution. For $\Sigma_{\eta'}/\Sigma_{\eta}$, we report the value, statistical error, and systematic error. The total error is the sum of the previous two in quadrature.

| Binning in $t$ ($\mathrm{GeV}^2$) | | | | Uncertainties | | |
|---|---|---|---|---|---|---|
| Range | Mean | RMS | $\Sigma_{\eta'}/\Sigma_{\eta}$ | Statistical | Systematic | Total |
| $0.1 < -t < 0.3$ | 0.206 | 0.061 | 0.868 | 0.067 | 0.033 | 0.075 |
| $0.3 < -t < 0.5$ | 0.392 | 0.056 | 0.942 | 0.082 | 0.034 | 0.088 |
| $0.5 < -t < 0.7$ | 0.589 | 0.056 | 0.956 | 0.109 | 0.072 | 0.131 |
| $0.7 < -t < 1.2$ | 0.883 | 0.136 | 1.077 | 0.120 | 0.040 | 0.126 |
